# Supplementary material for: Assembling a high-precision abundance catalogue of solar twins in GALAH for phylogenetic studies
Source: arXiv:2310.15107 source file (2024-01-24)
Supplement: Supplementary file 1 [file appendix_table_.tex]

\begin{table}
\begin{tabular}{|r|r|r|r|}
\hline
  \multicolumn{1}{|c|}{Tree ID} &
  \multicolumn{1}{c|}{Gaia DR3 ID} &
  \multicolumn{1}{c|}{Age} &
  \multicolumn{1}{c|}{Eccentricity} \\
\hline
  51 & 666015188409577984 & 9.78 & 0.4246\\
  52 & 6322247148827387136 & 6.87 & 0.4230\\
  53 & 5393131442215235200 & 9.17 & 0.4212\\
  54 & 601674104412705664 & 8.02 & 0.4210\\
  55 & 3883300178236623104 & 6.24 & 0.4196\\
  56 & 6667779157577097984 & 9.95 & 0.4194\\
  57 & 6405527900430451840 & 6.13 & 0.4194\\
  58 & 5279222175015479808 & 6.33 & 0.4181\\
  59 & 4757012868317667968 & 11.42 & 0.4179\\
  60 & 6478123572267779712 & 9.74 & 0.4177\\
  61 & 3883940094003907200 & 10.53 & 0.4172\\
  62 & 5638123901559960832 & 6.85 & 0.4152\\
  63 & 6308012424617699328 & 9.99 & 0.4144\\
  64 & 3287065366439298304 & 10.49 & 0.4142\\
  65 & 2557699964466229248 & 11.32 & 0.4135\\
  66 & 3614629431044065024 & 11.02 & 0.4130\\
  67 & 6085917569802394368 & 6.89 & 0.4127\\
  68 & 4733082826668647680 & 9.09 & 0.4125\\
  69 & 6282069752702417024 & 8.53 & 0.4123\\
  70 & 6765041750013972096 & 10.76 & 0.4118\\
  71 & 6423862810876918400 & 9.91 & 0.4107\\
  72 & 2725477089448504320 & 10.37 & 0.4100\\
  73 & 3540261075882678656 & 8.71 & 0.4094\\
  74 & 5946308592712694784 & 8.95 & 0.4090\\
  75 & 5566882729265564928 & 9.24 & 0.4088\\
  76 & 6271338282992948096 & 7.95 & 0.4088\\
  77 & 6684029385384375040 & 10.61 & 0.4079\\
  78 & 4086844214648752896 & 8.97 & 0.4077\\
  79 & 5381426659899459840 & 7.32 & 0.4077\\
  80 & 3185615352690802560 & 11.19 & 0.4076\\
  81 & 6219838773256412928 & 11.24 & 0.4069\\
  82 & 6112653913020941696 & 7.79 & 0.4053\\
  83 & 3595812320328032640 & 9.64 & 0.4051\\
  84 & 5279458668796971264 & 9.43 & 0.4048\\
  85 & 6145633729930145792 & 10.60 & 0.4046\\
  86 & 5403410948220358144 & 11.29 & 0.4044\\
  87 & 6138800540041985024 & 7.26 & 0.4044\\
  88 & 3252208064700926976 & 9.73 & 0.4029\\
  89 & 6470712760820762112 & 10.07 & 0.4028\\
  90 & 6403788717850875136 & 7.42 & 0.4025\\
  91 & 5224219621235036032 & 6.84 & 0.4023\\
  92 & 5500358736731918464 & 9.59 & 0.4014\\
  93 & 3468542578101858944 & 11.68 & 0.4012\\
  94 & 6358824189832315392 & 10.98 & 0.4009\\
  95 & 5394874576164852608 & 6.46 & 0.4008\\
  96 & 6358400534257921408 & 9.67 & 0.4007\\
  97 & 6888387232157424256 & 8.57 & 0.4005\\
  98 & 3554969620883294080 & 8.12 & 0.4002\\
  99 & 5668883976296706176 & 9.51 & 0.3998\\
  100 & 6380479243139810816 & 10.42 & 0.3996\\
  \hline
\end{tabular}
\caption{Stars selected for phylogenetic anaylisis. High eccentricity group stars 51-100.}\label{tab:selected_stars}
\end{table}

\begin{table}
\begin{tabular}{|r|r|r|r|}
\hline
  \multicolumn{1}{|c|}{Tree ID} &
  \multicolumn{1}{c|}{Gaia DR3 ID} &
  \multicolumn{1}{c|}{Age} &
  \multicolumn{1}{c|}{Eccentricity} \\
\hline
  101 & 6185629015145052672 & 7.18 & 0.0073\\
  102 & 5284653517640839168 & 8.05 & 0.0073\\
  103 & 3235925706241483520 & 6.42 & 0.0072\\
  104 & 6884833606280164736 & 9.19 & 0.0071\\
  105 & 3480132182276897024 & 3.07 & 0.0071\\
  106 & 5480059789282023040 & 6.61 & 0.0071\\
  107 & 6358142595701902208 & 9.12 & 0.0070\\
  108 & 5266820263672025728 & 3.64 & 0.0070\\
  109 & 6439049059324117248 & 5.00 & 0.0069\\
  110 & 6405046318633781376 & 8.88 & 0.0069\\
  111 & 5461297795883450368 & 5.91 & 0.0068\\
  112 & 50063964165971968 & 7.20 & 0.0068\\
  113 & 3810605799463298304 & 7.03 & 0.0068\\
  114 & 6682735539371249920 & 3.89 & 0.0067\\
  115 & 1739290475880215168 & 9.29 & 0.0066\\
  116 & 4710103171086624256 & 9.53 & 0.0066\\
  117 & 3487317834361589120 & 4.77 & 0.0066\\
  118 & 6364908509224429824 & 6.75 & 0.0066\\
  119 & 4733111345251454592 & 7.81 & 0.0064\\
  120 & 5483440478299224576 & 1.41 & 0.0063\\
  121 & 3223784379156708736 & 5.93 & 0.0063\\
  122 & 6088447408620627072 & 7.19 & 0.0063\\
  123 & 4694259689566847488 & 6.46 & 0.0062\\
  124 & 67653126552276224 & 5.12 & 0.0062\\
  125 & 6396608425885067008 & 6.97 & 0.0061\\
  126 & 6123111230667548800 & 6.16 & 0.0061\\
  127 & 5464025478071676800 & 6.36 & 0.0061\\
  128 & 6088768706533199616 & 6.43 & 0.0061\\
  129 & 4676886890452826112 & 7.14 & 0.0061\\
  130 & 5461908471511519488 & 9.46 & 0.0060\\
  131 & 5651004164883477632 & 5.45 & 0.0059\\
  132 & 4705870051319868032 & 10.84 & 0.0059\\
  133 & 4797809014612357760 & 9.35 & 0.0059\\
  134 & 4657140486320218112 & 10.52 & 0.0059\\
  135 & 6000803000315148416 & 7.38 & 0.0059\\
  136 & 2976255728739142656 & 4.02 & 0.0058\\
  137 & 5382523903786793472 & 9.90 & 0.0058\\
  138 & 6715094402798292480 & 3.41 & 0.0058\\
  139 & 5381323821202550272 & 3.16 & 0.0057\\
  140 & 5909353594569250048 & 4.54 & 0.0055\\
  141 & 3104341338654783488 & 9.70 & 0.0055\\
  142 & 6186327617345618816 & 4.39 & 0.0054\\
  143 & 4628586753393426560 & 2.48 & 0.0054\\
  144 & 6170081955088789760 & 7.08 & 0.0053\\
  145 & 4809907727029507072 & 5.90 & 0.0053\\
  146 & 6085188215637686656 & 7.46 & 0.0053\\
  147 & 4678732004106190208 & 8.78 & 0.0053\\
  148 & 5731489549907102976 & 3.60 & 0.0052\\
  149 & 4689717778831558656 & 4.80 & 0.0052\\
  150 & 5499064405387595648 & 8.38 & 0.0051\\
  \hline
\end{tabular}
\caption{Stars selected for phylogenetic anaylisis. Low eccentricity group stars 101-150.}
\end{table}

\begin{table}
\begin{tabular}{|r|r|r|r|}
\hline
  \multicolumn{1}{|c|}{Tree ID} &
  \multicolumn{1}{c|}{Gaia DR3 ID} &
  \multicolumn{1}{c|}{Age} &
  \multicolumn{1}{c|}{Eccentricity} \\
\hline
  151 & 6395166794341406592 & 7.82 & 0.0048\\
  152 & 5676142642826259968 & 4.35 & 0.0048\\
  153 & 4651467212427245696 & 3.87 & 0.0047\\
  154 & 5287550460200923648 & 6.42 & 0.0047\\
  155 & 5462907618345388544 & 2.90 & 0.0047\\
  156 & 5315596424848898560 & 4.59 & 0.0047\\
  157 & 6759872327379068672 & 4.53 & 0.0046\\
  158 & 4697080246129688448 & 6.56 & 0.0046\\
  159 & 3222243795862460544 & 5.01 & 0.0045\\
  160 & 5371299230102667008 & 9.43 & 0.0044\\
  161 & 6702072238057232768 & 6.82 & 0.0044\\
  162 & 6092999180602361600 & 4.75 & 0.0043\\
  163 & 5947687277209178624 & 2.91 & 0.0043\\
  164 & 5750202481897475456 & 5.04 & 0.0043\\
  165 & 5287639726800821248 & 4.07 & 0.0042\\
  166 & 3223509638687710080 & 3.53 & 0.0042\\
  167 & 4673758981733907072 & 9.45 & 0.0041\\
  168 & 6126830672354916096 & 7.82 & 0.0040\\
  169 & 5566278612049473152 & 5.04 & 0.0040\\
  170 & 6224013515831947136 & 6.54 & 0.0040\\
  171 & 5549974641315821312 & 6.84 & 0.0040\\
  172 & 602671876855711488 & 3.69 & 0.0039\\
  173 & 2581985874221363712 & 8.21 & 0.0039\\
  174 & 4795106999146072576 & 4.28 & 0.0038\\
  175 & 3466260438640320128 & 4.89 & 0.0037\\
  176 & 3486657444486961536 & 6.68 & 0.0037\\
  177 & 5442125096233286144 & 8.64 & 0.0036\\
  178 & 5222518298789556480 & 8.33 & 0.0035\\
  179 & 3858756918336549248 & 8.22 & 0.0034\\
  180 & 4705401006531314688 & 8.33 & 0.0033\\
  181 & 3609018932445213440 & 6.30 & 0.0033\\
  182 & 5797458735757029504 & 8.48 & 0.0033\\
  183 & 5025426475819519232 & 5.89 & 0.0032\\
  184 & 3086587150741484416 & 2.92 & 0.0032\\
  185 & 5261981862754043264 & 8.88 & 0.0029\\
  186 & 2891229773007818240 & 2.04 & 0.0028\\
  187 & 5673737014463160192 & 6.35 & 0.0028\\
  188 & 5808027928713875328 & 3.93 & 0.0028\\
  189 & 2595002133389005824 & 6.13 & 0.0027\\
  190 & 3201210447661057536 & 8.18 & 0.0024\\
  191 & 6044641284830208000 & 4.40 & 0.0024\\
  192 & 3482226034669980160 & 5.15 & 0.0022\\
  193 & 5485166711554949376 & 9.72 & 0.0022\\
  194 & 6137077364802632192 & 9.27 & 0.0020\\
  195 & 5269018397872024704 & 3.21 & 0.0019\\
  196 & 5375945525718174336 & 6.94 & 0.0017\\
  197 & 3220600232137213696 & 6.90 & 0.0014\\
  198 & 5374629719537552512 & 2.68 & 0.0013\\
  199 & 3458967137494974976 & 8.98 & 0.0010\\
  200 & 6140846937339223936 & 10.19 & 0.0007\\
\hline
\end{tabular}
\caption{Stars selected for phylogenetic anaylisis. Low eccentricity group stars 151-200.}
\end{table}
